# Supplementary material for: Tight Typings and Split Bounds
Source: arXiv:1807.02358 source file (2018-07-06)
Supplement: Supplementary file 2 [file toappendix.tex]

\gettoappendix {prop:tight-normal-forms-indicies}
\gettoappendix {l:tight-spreading-spi-ske}
\gettoappendix {l:typing-substitution-overview}
\gettoappendix {prop:subject-reduction}
\gettoappendix {thm:correctness}
\gettoappendix {prop:normal-forms-are-tightly-typable}
\gettoappendix {l:anti-substitution}
\gettoappendix {prop:subject-expansion}
\gettoappendix {thm:completeness}
\gettoappendix {prop:mxsubject-reduction}
\gettoappendix {prop:mxsubject-reductionproof}
\gettoappendix {prop:mxsubject-expansion}
\gettoappendix {prop:mxsubject-expansionproof}
\gettoappendix {prop:memory-bievaluation}
\gettoappendix {l:lin-head-headvar-in-context}
\gettoappendix {prop:tight-normal-forms-indicies-linear-head}
\gettoappendix {l:subst:hwmilner}
\gettoappendix {prop:head-subject-head-reduction}
\gettoappendix {tm:head-correctness}
\gettoappendix {prop:lin-head-normal-forms-are-tightly-typable}
\gettoappendix {l:anti-subst}
\gettoappendix {prop:linear-subject-expansion}
\gettoappendix {th:completeness-linear-head}
\gettoappendix {prop:shrinking-normal-forms-forall}
\gettoappendix {l:shrinking-neutral-spreading}
\gettoappendix {prop:shrinking-subject-reduction}
\gettoappendix {tm:shrinking-correctness}
\gettoappendix {prop:shrinking-normal-forms-exist}
\gettoappendix {prop:shrinking-subject-expansion}
\gettoappendix {thm:shrinking-completeness}
